# Supplementary material for: Optical Probes of the Quantum-Entangled Triplet-Triplet State in a Heteroacene Dimer
Source: arXiv:1809.09754 source file (2018-09-25)
Supplement: Supplementary file 1 [file SuppInfov5.pdf]

# Optical Probes of the Quantum-Entangled Triplet-Triplet State in a Heteroacene Dimer

## Supplemental Material

Souratosh Khan
*Department of Physics, University of Arizona Tucson, AZ 85721*

Sumit Mazumdar
*Department of Physics, University of Arizona*
*Department of Chemistry and Biochemistry, University of Arizona and*
*College of Optical Sciences, University of Arizona*
(Dated: September 25, 2018)

## A. TIPS-PENTACENE AND TIPS-TETRACENE

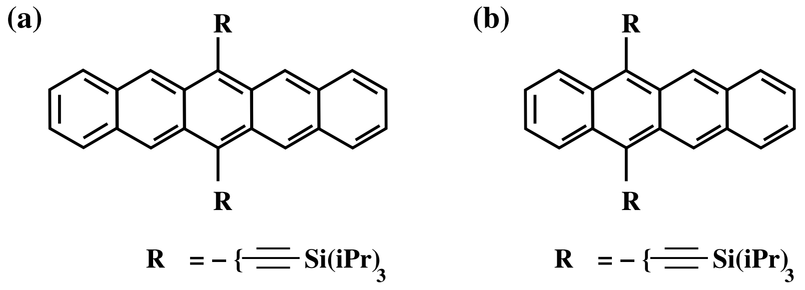


FIG. S1: (a) TIPS-pentacene molecule. (b) TIPS-tetracene molecule

TIPS-pentacene has both reflection (along the long and short axis) and center of inversion symmetries. As a consequence, the basis space belongs to the $D_{2h}$ point group symmetry Eigenstates can therefore classified as $A_g$, $B_{2u}$, $B_{3u}$ or $B_{1g}$ states. In contrast, TIPS-tetracene has a mirror-plane symmetry along the long axis of the molecule with $C_s$ symmetry. There is an additional charge conjugation symmetry which we ignore here for the sake of simplicity.

## B. MULTIPLE REFERENCE SINGLES AND DOUBLES CONFIGURATION INTERACTION (MRSDCI)

As discussed in the main text, once the HF basis MOs are obtained by solving the self-consistent equations to the PPP Hamiltonian, wavefunctions of the targeted excited states are constructed using the MRSDCI method in an iterative manner. In the first step, a trial set of singly and doubly excited configurations ($N_{ref}$) from the HF ground state constitute the configuration interaction matrix. The next step involves the inclusion of the most dominant triple and quadruple excitations from $N_{ref}$. This process is repeated till the most dominant single, double, triple and quadruple configurations with coefficients greater than 0.04 have been included in our calculation. The total size of the Hamiltonian is given by $N_{total}$. In Table I, we have listed $N_{ref}$ and $N_{total}$ for our calculations within the different symmetry subspaces of TIPS-P. $N_{ref}$ for QCI (quadruple CI) is left blank since it refers to the ground state configuration from which all possible single, double, triple and quadruple excitations are generated.

### I. TIPS-pentacene

TABLE S1: TIPS-pentacene : $N_{ref}$ and $N_{total}$ values in the different subspaces of the singlet and triplet manifolds.

| Parameters | | $^1A_g$ | $^1B_{2u}$ | $^1B_{3u}$ | $^3A_g$ | $^3B_{2u}$ | $^3B_{1g}$ |
|---|---|---|---|---|---|---|---|
| | Method | QCI | QCI | MRSDCI | MRSDCI | QCI | MRSDCI |
| **U = 6.7 eV, $\kappa$ = 1.0** | $N_{ref}$ | – | – | 104 | 87 | – | 78 |
| | $N_{total}$ | 1002823 | 1707547 | 346674 | 630871 | 3202443 | 512544 |
| | $N_{ref}$ | – | – | 86 | 72 | – | 94 |
| **U = 7.7 eV, $\kappa$ = 1.3** | $N_{total}$ | 1002823 | 1707547 | 324326 | 721575 | 3202443 | 679048 |

### II. TIPS-tetracene

Our calculations for TIPS-tetracene do not use any symmetry. The sizes of the singlet and triplet hamiltonian matrices using the QCI method are 4006553 and 12826581, respectively.

## III. PTn

TABLE S2: $N_{ref}$ and $N_{total}$ values determined in the calculation of the ground and excited state absorption spectra in PT0, PT1 and PT2.

| Transition | PT0 | | | | PT1 | | | | PT2 | | | |
|---|---|---|---|---|---|---|---|---|---|---|---|---|
| | U = 6.7 eV $\kappa$ = 1.0 | | U = 7.7 eV $\kappa$ = 1.3 | | U = 6.7 eV $\kappa$ = 1.0 | | U = 7.7 eV $\kappa$ = 1.3 | | U = 6.7 eV $\kappa$ = 1.0 | | U = 7.7 eV $\kappa$ = 1.3 | |
| | $N_{ref}$ | $N_{total}$ | $N_{ref}$ | $N_{total}$ | $N_{ref}$ | $N_{total}$ | $N_{ref}$ | $N_{total}$ | $N_{ref}$ | $N_{total}$ | | |
| $S_0 \rightarrow S_1$ | 163 | 2884542 | – | – | 230 | 3978477 | – | – | – | – | – | – |
| $S_1 \rightarrow S_N$ | 248 | 3582257 | – | – | 167 | 2890316 | – | – | – | – | – | – |
| $T_1 \rightarrow T_N$ | 116 | 1843555 | 113 | 2053573 | 134 | 2305628 | 151 | 2621463 | 142 | 2570116 | 153 | 2830133 |
| $^1(TT)_1 \rightarrow {}^1(TT)_N$ | 262 | 3871072 | 249 | 3839640 | 298 | 3900193 | 300 | 4163370 | 235 | 3282779 | 226 | 3823065 |

## C. MONOMER CALCULATION RESULTS

TABLE S3: Experimental versus calculated energies of the lowest singlet and triplet excitons, and the lowest triplet transition energy in eV, for TIPS-pentacene.

| State | Expt | U = 6.7 eV $\kappa$ = 1.0 | U = 7.7 eV $\kappa$ = 1.3 |
|---|---|---|---|
| $S_1$ | 1.81, 1.9 | 1.88 | 2.22 |
| $T_1$ | $\sim$ 0.95 | 0.90 | 0.89 |
| $T_3 - T_1$ | $\sim$ 2.46 | 2.1 | 2.39 |

TABLE S4: Experimental versus calculated energies of the lowest singlet and triplet excitons, and the lowest triplet transition energy in eV, for TIPS-tetracene.

| State | Expt | U = 6.7 eV $\kappa$ = 1.0 | U = 7.7 eV $\kappa$ = 1.3 |
|---|---|---|---|
| $S_1$ | 2.3 | 2.19 | 2.57 |
| $T_1$ | $\sim$ 1.25 | 1.16 | 1.06 |
| $T_3 - T_1$ | $\sim$ 2.92 | 3.35 | 3.56 |

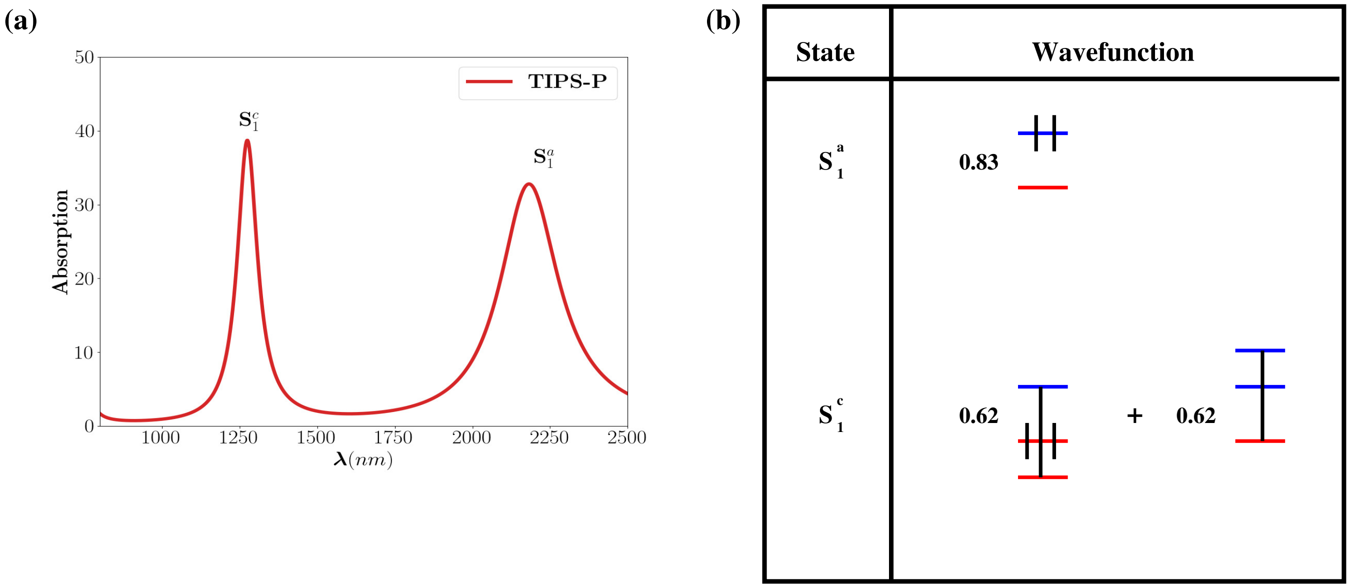


FIG. S2: (a) Singlet ESA in the TIPS-P monomer in SWIR region with $U = 6.7$ eV, $\kappa = 1.0$. The final states are labeled $S_1^a$ and $S_1^c$. (b) Dominant contributions to the wavefunctions of the final states show that $S_1^a$ is composed of HOMO, HOMO $\rightarrow$ LUMO, LUMO 2e-2h excitations while $S_1^c$ is given by HOMO (HOMO-1) $\rightarrow$ LUMO+1 (LUMO) transitions. These absorptions appear in PTn as well (see Fig. S3 and main text).

## D. PTn CALCULATION RESULTS

### I. $S_1$,$S_2$ and $S_3$ wavefunctions

The optical wavefunctions. $S_1$ and $S_2$ are localized on pentacene and tetracene, respectively, in both PT0 and PT1. $S_3$ is CT with equal contributions from pentacene $\rightarrow$ tetracene as well as its counterpart. In PT1, excitations between the bonding MOs of pentacene/tetracene to the anti-bonding MOs of phenyl linker have non-negligible contributions. There exists an optically allowed $S_4$ state (not shown) close to 3.3 eV in both PT0 and PT1 that is primarily composed of excitations within the tetracene molecule.

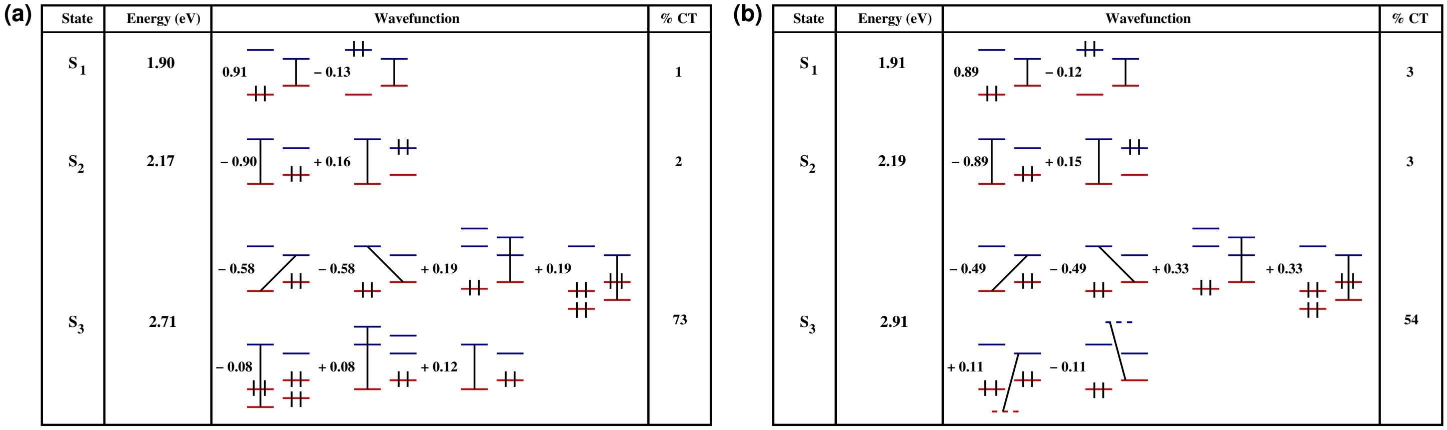


FIG. S3: Dominant contributions to the wavefunctions of the lowest singlet optical states in (a) PT0 and (b) PT1 for $U = 6.7$ eV, $\kappa = 1.0$. The solid red (blue) lines are the bonding (anti-bonding) MOs that are localized on the pentacene and tetracene units of the molecule. The dashed lines represent the single particle energy levels that reside on the benzene ring in PT1. While almost 80% of the weight in $S_1$ ($S_2$) comes from a HOMO $\rightarrow$ LUMO excitation within the TIPS-P (TIPS-T) subunit, the remaining 20% in both PT0 and PT1 consist of mostly localized higher order excitations within the subunits; the contribution from HOMO $\rightarrow$ LUMO 1e-1h excitation on the other unit is zero.

## II. Singlet Excited State Absorption (ESA)

Given below is the singlet ESA in the PT0 and PT1 dimers (see Fig. S4). Due to computational limitations the spectra of PT1 can be calculated in NIR and SWIR regions only.

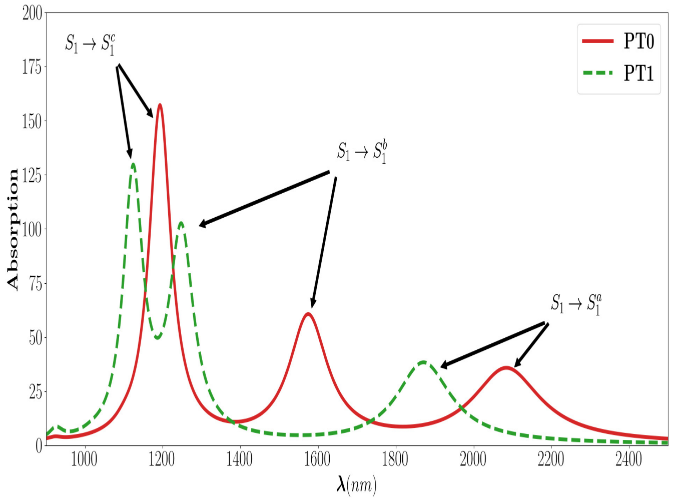


FIG. S4: Calculated singlet ESA from $S_1$ in PT0 (solid red) and PT1 (dashed green) with $U$ = 6.7 eV, $\kappa$ = 1.0 beyond the visible region.

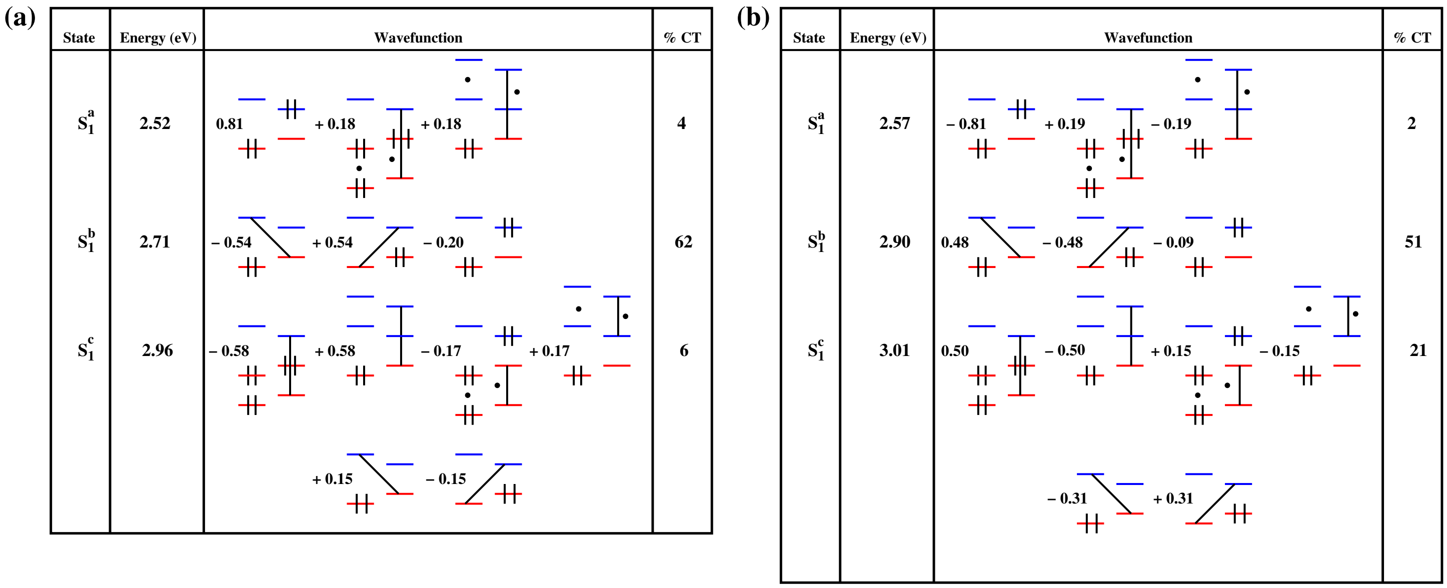


FIG. S5: Dominant contributions to the wavefunctions of the final states $S_1^a$, $S_1^b$ and $S_1^c$ in calculated singlet ESA spectra of (a) PT0 and (b) PT1 with with $U = 6.7$ eV, $\kappa = 1.0$ in NIR and SWIR. Dots between MOs indicate the presence of other MOs in between.

## III. $T_1$, $T_2$, $T_3$ and $T_4$ wavefunctions: PT0 and PT1

Below, we present the energies, wavefunctions and the degree of CT of $T_1$, $T_2$, $T_3$ and $T_4$ in PT0 and PT1.

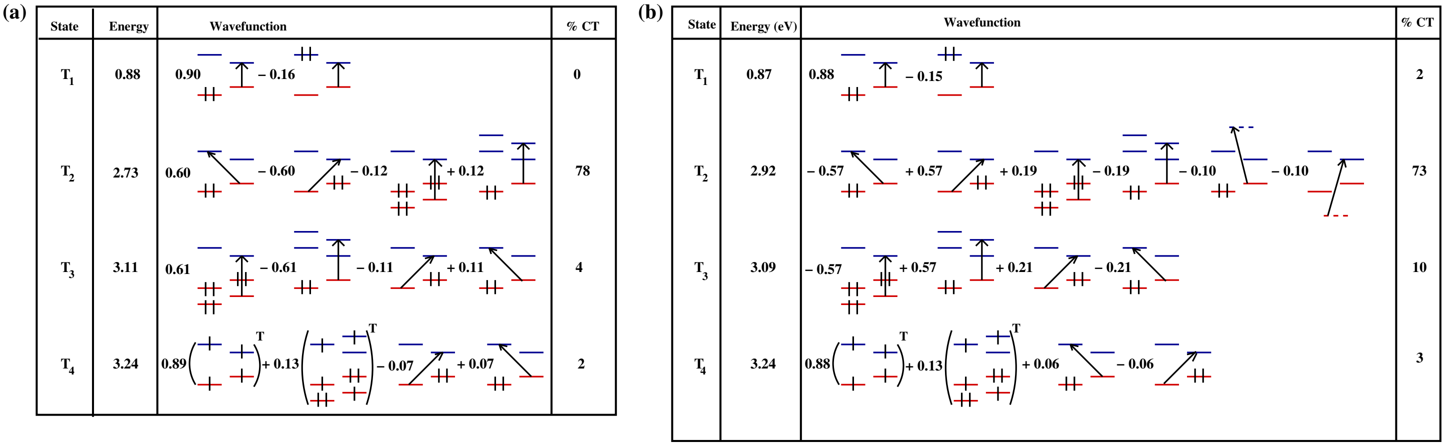


FIG. S6: Dominant contributions to the wavefunctions of the lowest triplet excited states $T_1$ - $T_4$ to which triplet ESAs occur, (a) PT0 and (b) PT1 ($U$ = 7.7 eV, $\kappa$ = 1.3).

## IV. Triplet ESA

Sensitization experiments carried out by Sanders *et al.* (see reference 15 in main text) lead to long lasting triplet excitons on both pentacene ($T_1$) and tetracene ($T'_1$) subunits in PTn. The calculated triplet ESA spectra from the two units are overlapping (see Fig. S7) with the intensity of $T'_1 \rightarrow T_N$ transitions being significantly weaker than the corresponding transitions from $T_1$.

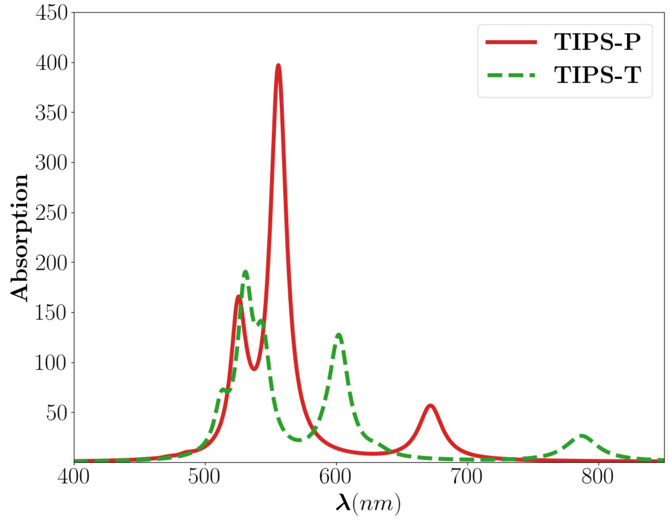


FIG. S7: Calculated triplet ESA from $T_1$ (triplet localized on TIPS-P - solid red) and $T'_1$ (triplet localized on TIPS-T - dashed green) in PT0 with $U$ = 7.7 eV, $\kappa$ = 1.3. The calculations of the absorptions in the two molecules use the same units, such that their relative oscillator strengths are as indicated as in the figure.

## V. The Triplet-Triplet state in PTn

The energies of the $^1(TT)_1$ states are 1.97 eV, 2.00 eV and 2.07 eV in PT0, PT1 and PT2, respectively. Fig. S8 gives the most dominant contributions to the $^1(TT)_1$ wavefunction in PTn (n = 0, 1 and 2). In all the three dimers, the 2e-2h excited configuration that is a product state of two triplets and that constitutes nearly 80% of the overall wavefunction are localized on the acene monomer units. We find very little contribution from the benzene MOs in the $^1(TT)_1$ states. The convergence of the triplet and $^1(TT)_1$ ESA spectra in the visible region and the reduced intensity

of the $^1$(TT)$_1$ $\rightarrow$ S$_3$ transition in PT1 and PT2 signal a decrease in the quantum entanglement of $^1$(TT)$_1$ in dimers with large n (see Figs. 6, 7 of main text).

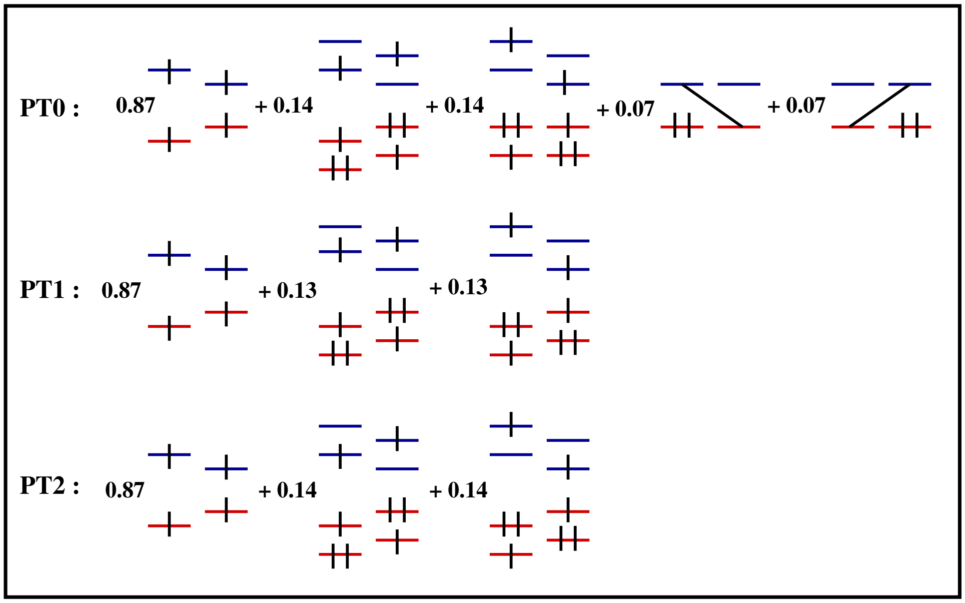


FIG. S8: The $^1$(TT)$_1$ states in PT0, PT1 nd PT2 for $U = 7.7$ eV and $\kappa = 1.3$.
